# Supplementary material for: Perfect Generation of Angular Momentum with Cylindrical Bianisotropic Metasurfaces
Source: arXiv:1806.04349 source file (2018-06-12)
Supplement: Supplementary file 1 [file Supp_Mat.pdf]

**Supplementary material for the paper**

# "Perfect Generation of Angular Momentum with Cylindrical Bianisotropic Metasurfaces"

Junfei Li, Ana Díaz-Rubio, Chen Shen, Zhetao Jia, Sergei Tretyakov, and Steven Cummer

## SUPPLEMENTARY NOTE 1: Electromagnetic formulation

Using a similar analysis to that the proposed in the main text, metasurfaces for perfect cylindrical transformations of electromagnetic wavefronts can be designed. For example, let us consider the TE-polarization case where electric field along $z$-direction, $\mathbf{E} = E_z\hat{z}$. The wave equation for TE-polarization can be written as

$$\frac{1}{r}\frac{\partial}{\partial r}\left(\frac{\partial E_z}{\partial r}\right) + \frac{1}{r^2}\frac{\partial^2 E_z}{\partial \varphi^2} = \frac{1}{c_0^2}\frac{\partial^2 E_z}{\partial t^2}. \quad (1)$$

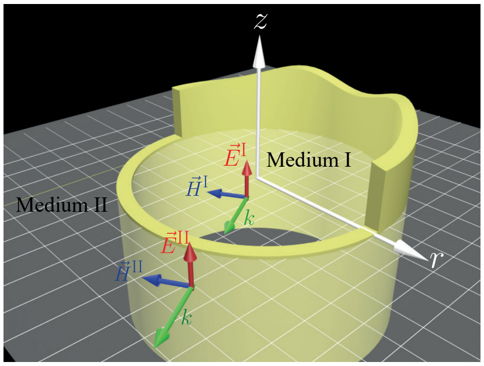


**Supplementary Figure 1:** Schematic representation electromagnetic system for TE-polarization.

It is clear that this wave equation has the same form than the acoustic counterpart and consequently the solution can also be expressed as a combination of cylindrical waves emerging $[H_n^{(1)}(kr)]$ and diverging $[H_n^{(2)}(kr)]$ from the origin of coordinates with a certain angular momentum $n$.

We start defining a diverging wave with angular momentum, $n_1$, in the Medium I that can be written as

$$E_z^{\mathrm{I}} = E_0 H_{n1}^{(2)}(kr)e^{jn_1\varphi}, \quad (2)$$

where $E_0$ is the amplitude of the wave. It is easy to obtain the expression of the corresponding magnetic field by applying Maxwell equation ($\nabla \times \mathbf{E} = -j\omega\mu_0\mathbf{H}$). Finally, the magnetic field reads

$$\mathbf{H}^{\mathrm{I}} = -\frac{E_0}{Z_0}\left[\frac{n_1}{kr}H_{n1}^{(2)}(kr)\hat{r} + j\partial_r H_{n1}^{(2)}(kr)\hat{\varphi}\right]e^{jn_1\varphi}, \quad (3)$$

with $Z_0 = \sqrt{\mu_0/\varepsilon_0}$ being the wave impedance in the background field. Following the same approach, the field in Medium II will be defined as

$$E_z^{\mathrm{II}} = E_{\mathrm{t}} H_{n2}^{(2)}(kr)e^{jn_2\varphi}, \quad (4)$$

where $T$ is the transmission coefficient and $n_2$ is the angular momentum of the fields outside the metasurface. The expressions for the magnetic field in the Medium II is

$$\mathbf{H}^{\mathrm{II}} = \frac{E_{\mathrm{t}}}{Z_0}\left[\frac{n_2}{kr}H_{n2}^{(2)}(kr)\hat{r} + j\partial_r H_{n2}^{(2)}(kr)\hat{\varphi}\right]e^{jn_2\varphi}. \quad (5)$$

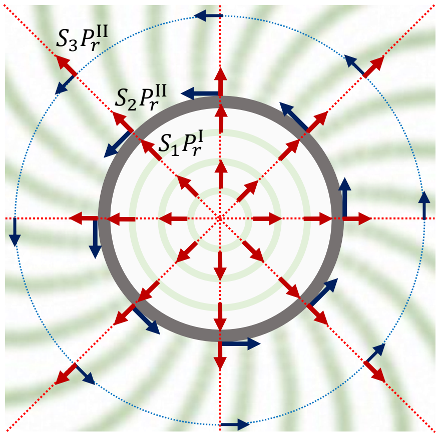


**Supplementary Figure 2:** Schematic representation of the Poynting vector distribution inside and outside the metasurface. Green patterns represent the wavefronts.

In order to realize perfect cylindrical transformations, it is necessary to ensure the fulfillment of the power conservation between the waves inside and outside the metasurface. The Poynting vector of the cylindrical waves can be calculated as $\vec{P} = \frac{1}{2}\mathrm{Re}\left\{\vec{E} \times \vec{H}^*\right\} = P_r\hat{r} + P_\varphi\hat{\varphi}$, where

$$P_r = \frac{E_0^2}{\pi Z_0}\frac{1}{r} \tag{6}$$

and

$$P_\varphi = \frac{E_0^2}{\pi Z_0}\frac{n}{kr}J_n(kr). \tag{7}$$

The angular component of the Poynting vector, $P_\varphi$, represents the with circulated around the origin of coordinates (see Figure 2). Due to the inherent periodicity of the system in the angular direction, this component do not contribute to the global power balance. If we consider that the internal and external boundaries of the metasurface are located at $r_1$ and $r_2$, the condition for ensuring the power balance reads $S_1P_r^{\mathrm{I}}|_{r_1} = S_2P_r^{\mathrm{II}}|_{r_2}$. Finally, the amplitude of incident transmitted waves should satisfy $E_{\mathrm{t}} = E_0$.

Once the desired waves are fully defined, one has to relate the fields at both sides of the metasurface as follows

$$\begin{bmatrix} E^{\mathrm{I}}(r_1,\varphi) \\ E^{\mathrm{II}}(r_2,\varphi) \end{bmatrix} = \begin{bmatrix} Z_{11} & Z_{12} \\ Z_{12} & Z_{22} \end{bmatrix} \begin{bmatrix} S_1\hat{n} \times H^{\mathrm{I}}(r_1,\varphi) \\ -S_2\hat{n} \times H^{\mathrm{II}}(r_1,\varphi) \end{bmatrix} \tag{8}$$

where $\hat{n}$ is the normal vector to the metasurface and the matrix $[Z]$ defines the electromagnetic properties of the metasurface. It is important to notice that the off-diagonal terms of the impedance matrix are force to be equal, meaning that we will inspect only reciprocal metasurfaces. In addition to the reciprocal condition, we will impose the lossless behavior by considering all the element of the impedance matrix pure-imaginary, $Z_{ij} = jX_{ij}$. The equation system can be expressed as

$$\begin{cases} Z_0C_{n_1} = -S_1X_{11}C'_{n_1} + S_2X_{12}C'_{n_2} \\ Z_0C_{n_2} = -S_1X_{12}C'_{n_1} + S_2X_{22}C'_{n_2} \end{cases} \tag{9}$$

where

$$C_{n_1} = H_{n_1}^{(2)}(kr_1)e^{\mathrm{j}n_1\phi} \tag{10}$$

$$C'_{n_1} = \frac{1}{2}[H_{n_1-1}^{(2)}(kr_1) - H_{n_1+1}^{(2)}(kr_1)]e^{\mathrm{j}n_1\phi} \tag{11}$$

$$C_{n_2} = H_{n_2}^{(2)}(kr_2)e^{\mathrm{j}n_2\phi} \tag{12}$$

$$C'_{n_2} = \frac{1}{2}[H_{n_2-1}^{(2)}(kr_2) - H_{n_2+1}^{(2)}(kr_2)]e^{\mathrm{j}n_2\phi} \tag{13}$$

After some algebra, the components in the impedance matrix can thus be calculated:

$$X_{11} = -\frac{Z_0}{S_1}\frac{\mathrm{Im}(C'_{n_1})\mathrm{Re}(C_{n_2}) - \mathrm{Re}(C'_{n_2})\mathrm{Im}(C_{n_1})}{\mathrm{Im}(C'_{n_2})\mathrm{Re}(C'_{n_1}) - \mathrm{Re}(C'_{n_2})\mathrm{Im}(C'_{n_1})} \tag{14}$$

$$X_{22} = \frac{Z_0}{S_2}\frac{\mathrm{Im}(C_{n_2})\mathrm{Re}(C'_{n_1}) - \mathrm{Re}(C_{n_2})\mathrm{Im}(C'_{n_1})}{\mathrm{Im}(C'_{n_2})\mathrm{Re}(C'_{n_1}) - \mathrm{Re}(C'_{n_2})\mathrm{Im}(C'_{n_1})} \tag{15}$$

$$X_{12} = -\frac{Z_0}{S_1}\frac{2}{\pi r_2}\frac{1}{\mathrm{Im}(C'_{n_2})\mathrm{Re}(C'_{n_1}) - \mathrm{Re}(C'_{n_2})\mathrm{Im}(C'_{n_1})} \tag{16}$$

## SUPPLEMENTARY NOTE 2: Transfer matrix of a sector of wedge-shaped material

**Acoustic waves and TE-polarized electromagnetic waves**. Here we consider an acoustic notation as an example (for TE-polarized EM waves, the results are equivalent). The fields generated by a monopole source located at the center can be written as

$$p = XH_0^{(2)}(kr) + YH_0^{(1)}(kr) \tag{17}$$

$$v = -\frac{1}{2\mathrm{j}Z_0}\{X[H_{-1}^{(2)}(kr) - H_1^{(2)}(kr)] + Y[H_{-1}^{(1)}(kr) - H_1^{(1)}(kr)]\} \tag{18}$$

The transfer matrix is defined as

$$\begin{bmatrix} p_i \\ S_1 v_i \end{bmatrix} = \begin{bmatrix} M_{11} & M_{12} \\ M_{21} & M_{22} \end{bmatrix} \begin{bmatrix} p_o \\ S_2 v_o \end{bmatrix}. \tag{19}$$

where the subscripts denote the fields at the input port $r_1$ and output port $r_2$. To calculate these values, we first impose that $v_o = 0$, so that $M_{11} = p_i/p_o$ and $M_{21} = S_1 v_i/p_o$. This condition is satisfied when

$$\frac{Y}{X} = \alpha = -\frac{H_{-1}^{(2)}(kr_2) - H_1^{(2)}(kr_2)}{H_{-1}^{(1)}(kr_2) - H_1^{(1)}(kr_2)} \tag{20}$$

Then $M_{11}$ and $M_{21}$ can be calculated as

$$M_{11} = \frac{H_0^{(2)}(kr_1) + \alpha H_0^{(1)}(kr_1)}{H_0^{(2)}(kr_2) + \alpha H_0^{(1)}(kr_2)} \tag{21}$$

$$M_{21} = -\frac{S_1}{2\mathrm{j}Z_0}\frac{H_{-1}^{(2)}(kr_1) - H_1^{(2)}(kr_1) + \alpha[H_{-1}^{(1)}(kr_1) - H_1^{(1)}(kr_1)]}{H_0^{(2)}(kr_2) + \alpha H_0^{(1)}(kr_2)} \tag{22}$$

Similarly, we can impose that $p_o = 0$, so that $M_{12} = p_i/S_2 v_o$ and $M_{22} = S_1 v_i/S_2 v_o$. This condition is satisfied when

$$\frac{Y}{X} = \beta = -\frac{H_0^{(2)}(kr_2)}{H_0^{(1)}(kr_2)} \tag{23}$$

Then $M_{12}$ and $M_{22}$ can be calculated as

$$M_{12} = -\frac{2jZ_0}{S_2}\frac{H_0^{(2)}(kr_1)+\beta H_0^{(1)}(kr_1)}{H_{-1}^{(2)}(kr_2)-H_1^{(2)}(kr_2)+\beta[H_{-1}^{(1)}(kr_2)-H_1^{(1)}(kr_2)]} \tag{24}$$

$$M_{22} = \frac{S_1}{S_2}\frac{H_{-1}^{(2)}(kr_1)-H_1^{(2)}(kr_1)+\beta[H_{-1}^{(1)}(kr_1)-H_1^{(1)}(kr_1)]}{H_{-1}^{(2)}(kr_2)-H_1^{(2)}(kr_2)+\beta[H_{-1}^{(1)}(kr_2)-H_1^{(1)}(kr_2)]} \tag{25}$$

Hence the transfer matrices can be calculated by assigning the corresponding input and output positions.

## SUPPLEMENTARY NOTE 3: Multilayer model for cylindrical bianisotropic metasurfaces

The analysis of a cylindrical metasurfaces with infinitesimal thickness capable of perfectly transforming the scattered wavefronts shows that bianisotropic response is needed. Such response can be obtained by controlling the electromagnetic coupling for EM waves or the Willis coupling in the acoustic counterpart. Looking into the scattering characteristic of such particles, one can see that the bianisotropic response is translated into asymmetric reflection from the backward and forward directions (same magnitude but different phases). Due to the small size required for the implementation of bianisotropic gradient metasurfaces, an extended way to fully control the asymmetric response of the particles is to cascade multiple metasurfaces.

### Electromagnetic metasurfaces

For the electromagnetic case, one can consider a cascade of metallic pattern separated by concentric dielectric substrates [see Figure 3]. The pattered metallic sheets can be modelled as shunt impedances with the following transfer matrix

$$M_{Zi} = \begin{bmatrix} 1 & 0 \\ Y_i & 1 \end{bmatrix}, i = 1,2,3 \tag{26}$$

where $Y_i = 1/Z_i$ represents the effective impedance of the metallic patterns. On the other hand the transmission matrix of the of a wedge-shaped dielectric sector can be expressed as

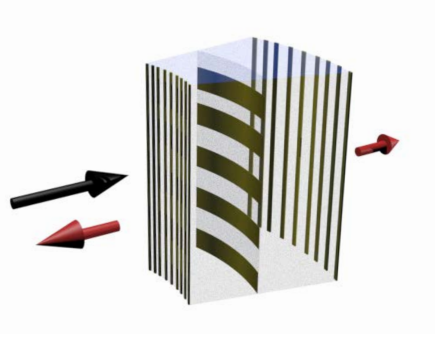

**Supplementary Figure 3:** Schematic representation of a multilayer system with fully controllable asymmetric response.

$$M_{Ti} = \begin{bmatrix} A_i & B_i \\ C_i & D_i \end{bmatrix}, i = 1,2 \tag{27}$$

The values matrix elements are functions of the inner and outer radius and the dielectric permittivity $\varepsilon_d$ (see Supplementary Note 2 for more information). Finally the total transmission matrix can be calculated

as

$$M = \begin{bmatrix} M_{11} & M_{12} \\ M_{21} & M_{22} \end{bmatrix} = M_{Z1} M_{T1} M_{Z2} M_{T2} M_{Z3} \tag{28}$$

After some algebra, we can obtain the required sheet admittances ($Y_1$, $Y_2$, and $Y_3$) as a function of the required scattering properties ($M_{11}$, $M_{12}$, $M_{21}$, and $M_{22}$)

$$Y_2 = \frac{M_{12} - B_1 D_2 - A_1 B_2}{B_1 B_2} \tag{29}$$

$$Y_1 = \frac{M_{22} - (D_1 D_2 + C_1 B_2 + D_1 B_2 Y_2)}{A_1 B_2 + B_1 D_2 + B_1 B_2 Z_2} \tag{30}$$

$$Y_3 = \frac{M_{11} - (B_1 C_2 + A_1 A_2 + B_1 A_2 Y_2)}{A_1 B_2 + B_1 D_2 + B_1 B_2 Y_2} \tag{31}$$

At microwave frequency the required sheet admittances can be implemented by using metallic patterns [1]

## Acoustic models

For the acoustic scenario, the asymmetric response can be obtained as cascade of three different membranes separated a certain distance. The response of a meta-atom can be expressed in terms of the transmission matrices

$$M = M_{Z1} M_{T1} M_{Z2} M_{T2} M_{Z3} \tag{32}$$

with

$$M_{Zi} = \begin{bmatrix} 1 & Z_i \\ 0 & 1 \end{bmatrix}, i = 1, 2, 3 \tag{33}$$

and $M_{Ti}, i = 1, 2$ is the transfer matrix of a wedge-shaped dielectric sector, which is a function of its inner and outer radius. Detailed derivation of the explicit expression of $M_{Ti}$ can be found in Supplementary Note 2. Here for simplicity, let us denote

$$M_{Ti} = \begin{bmatrix} A_i & B_i \\ C_i & D_i \end{bmatrix}, i = 1, 2 \tag{34}$$

Then the required impedances for the three membranes can be calculated as

$$Z_2 = \frac{M_{21} - C_1 A_2 - D_1 C_2}{C_1 C_2} \tag{35}$$

$$Z_1 = \frac{M_{11} - (A_1 A_2 + B_1 C_2 + A_1 C_2 Z_2)}{C_1 A_2 + D_1 C_2 + C_1 C_2 Z_2} \tag{36}$$

$$Z_3 = \frac{M_{22} - (C_1 B_2 + D_1 D_2 + C_1 D_2 Z_2)}{C_1 A_2 + D_1 C_2 + C_1 C_2 Z_2} \tag{37}$$

## SUPPLEMENTARY NOTE 4: Conversion from scattering matrix to transfer matrix

The transfer matrix of an arbitrary structure in a wedge-shaped waveguide is defined in Eq. (19), and the scattering matrix is

$$\begin{bmatrix} B \\ C \end{bmatrix} = \begin{bmatrix} S_{11} & S_{12} \\ S_{21} & S_{22} \end{bmatrix} \begin{bmatrix} A \\ D \end{bmatrix}. \tag{38}$$

Calculation strategy of the transfer matrix is the same as in Supp. Note 2, where we first set $v_o = 0$ to obtain $M_{11}$ and $M_{21}$. In this case we have $\frac{D}{C} = \alpha$ and

$$\frac{A}{C} = \frac{1 - S_{22}\alpha}{S_{21}} \tag{39}$$

$$\frac{B}{C} = \frac{1 - S_{22}\alpha}{S_{21}} S_{11} + S_{12}\alpha \tag{40}$$

where $\alpha$ is defined in Eq.(20). Then $M_{11}$ and $M_{21}$ can be expressed in terms of S matrix:

$$M_{11} = \frac{(1 - S_{22}\alpha)H_0^{(2)}(kr_1) + (S_{11} - S_{11}S_{22}\alpha + S_{21}S12\alpha)H_0^{(1)}(kr_1)}{S_{21}H_0^{(2)}(kr_2) + S_{21}\alpha H_0^{(1)}(kr_2)} \tag{41}$$

$$M_{21} = -\frac{S_1}{2\mathrm{j}Z_0} \frac{(1 - S_{22}\alpha)[H_{-1}^{(2)}(kr_1) - H_1^{(2)}(kr_1)] + (S_{11} - S_{11}S_{22}\alpha + S_{21}S12\alpha)[H_{-1}^{(1)}(kr_1) - H_1^{(1)}(kr_1)]}{S_{21}H_0^{(2)}(kr_2) + S_{21}\alpha H_0^{(1)}(kr_2)} \tag{42}$$

Similarly, we can impose that $p_o = 0$, in which case

$$\frac{A}{C} = \frac{1 - S_{22}\beta}{S_{21}} \tag{43}$$

$$\frac{B}{C} = \frac{1 - S_{22}\beta}{S_{21}} S_{11} + S_{12}\beta \tag{44}$$

where $\beta$ is defined in Eq.(23).so that $M_{12} = p_i/S_2 v_o$ and $M_{22} = S_1 v_i/S_2 v_o$ can be expressed as

$$M_{12} = -\frac{2\mathrm{j}Z_0}{S_2} \frac{(1 - S_{22}\beta)H_0^{(2)}(kr_1) + (S_{11} - S_{11}S_{22}\beta + S_{21}S12\beta)H_0^{(1)}(kr_1)}{S_{21}[H_{-1}^{(2)}(kr_2) - H_1^{(2)}(kr_2)] + S_{21}\beta[H_{-1}^{(1)}(kr_2) - H_1^{(1)}(kr_2)]} \tag{45}$$

$$M_{22} = \frac{S_1}{S_2} \frac{(1 - S_{22}\beta)[H_{-1}^{(2)}(kr_1) - H_1^{(2)}(kr_1)] + (S_{11} - S_{11}S_{22}\beta + S_{21}S12\beta)[H_{-1}^{(1)}(kr_1) - H_1^{(1)}(kr_1)]}{S_{21}[H_{-1}^{(2)}(kr_2) - H_1^{(2)}(kr_2)] + S_{21}\beta[H_{-1}^{(1)}(kr_2) - H_1^{(1)}(kr_2)]} \tag{46}$$

## SUPPLEMENTARY NOTE 5: Calculation of the matrices in the simulation

For the ease of implementation, the method we used to retrieve the impedance matrix in COMSOL is inspired by the standard 4-microphone method for acoustic experiments with impedance tubes, whose setups are shown in Fig. ?. The waves in the upstream and downstream can be written as

$$p_{\text{up}} = AH_0^{(2)}(kr) + AH_0^{(1)}(kr) \tag{47}$$

$$p_{\text{down}} = CH_0^{(2)}(kr) + DH_0^{(1)}(kr) \tag{48}$$

The positions of 4 microphones are $x_1$, $x_2$, $x_3$, $x_4$, respectively. By performing two measurements with different boundary conditions at the end of the tube, we can obtain four independent equations for determination of the four transfer matrix elements. Two different boundaries we used at the end of the tube are plane wave radiation (condition #1) and hard wall (condition #2). The pressure detected by these microphones under these two boundary conditions are noted as $p_m^{(n)}$ where $m$ denotes the number of the microphone and $n$ denotes the number of the boundary condition.They satisfy the condition:

$$\begin{bmatrix} H_0^{(2)}(kx_1) & H_0^{(1)}(kx_1) \\ H_0^{(2)}(kx_2) & H_0^{(1)}(kx_2) \end{bmatrix} \begin{bmatrix} A^{(1)} & A^{(2)} \\ B^{(1)} & B^{(2)} \end{bmatrix} = \begin{bmatrix} p_1^{(1)} & p_1^{(2)} \\ p_2^{(1)} & p_2^{(2)} \end{bmatrix} \tag{49}$$

Similarly,

$$\begin{bmatrix} H_0^{(2)}(kx_3) & H_0^{(1)}(kx_3) \\ H_0^{(2)}(kx_4) & H_0^{(1)}(kx_4) \end{bmatrix} \begin{bmatrix} C^{(1)} & C^{(2)} \\ D^{(1)} & D^{(2)} \end{bmatrix} = \begin{bmatrix} p_3^{(1)} & p_3^{(2)} \\ p_4^{(1)} & p_4^{(2)} \end{bmatrix} \tag{50}$$

With the measurement of $p_m^{(n)}$ under two different conditions, all the ABCD in the matrices can be calculated. Therefore, the scattering matrix can be calculated as

$$S = \begin{bmatrix} B^{(1)} & B^{(2)} \\ C^{(1)} & C^{(2)} \end{bmatrix} \begin{bmatrix} A^{(1)} & A^{(2)} \\ D^{(1)} & D^{(2)} \end{bmatrix}^{-1} \tag{51}$$

If the inner radius and outer radius of the metasurface is $r_1$ and $r_2$, then the pressure and volume velocity at both sides can be written as:

$$\begin{bmatrix} p_i^{(1)} & p_i^{(2)} \\ S_1 v_i^{(1)} & S_1 v_i^{(2)} \end{bmatrix} = \begin{bmatrix} H_0^{(2)}(kr_1) & H_0^{(1)}(kr_1) \\ -\frac{S_1}{2\mathrm{j}Z_0}[H_{-1}^{(2)}(kr_1) - H_1^{(2)}(kr_1)] & -\frac{S_1}{2\mathrm{j}Z_0}[H_{-1}^{(1)}(kr_1) - H_1^{(1)}(kr_1)] \end{bmatrix} \begin{bmatrix} A^{(1)} & A^{(2)} \\ B^{(1)} & B^{(2)} \end{bmatrix} \tag{52}$$

$$\begin{bmatrix} p_o^{(1)} & p_o^{(2)} \\ S_2 v_o^{(1)} & S_2 v_o^{(2)} \end{bmatrix} = \begin{bmatrix} H_0^{(2)}(kr_2) & H_0^{(1)}(kr_2) \\ -\frac{S_2}{2\mathrm{j}Z_0}[H_{-1}^{(2)}(kr_2) - H_1^{(2)}(kr_2)] & -\frac{S_2}{2\mathrm{j}Z_0}[H_{-1}^{(1)}(kr_2) - H_1^{(1)}(kr_2)] \end{bmatrix} \begin{bmatrix} C^{(1)} & C^{(2)} \\ D^{(1)} & D^{(2)} \end{bmatrix} \tag{53}$$

The transfer matrix of the measured unit cell can thus be calculated as

$$T = \begin{bmatrix} p_o^{(1)} & p_o^{(2)} \\ S_2 v_o^{(1)} & S_2 v_o^{(2)} \end{bmatrix} \begin{bmatrix} p_i^{(1)} & p_i^{(2)} \\ S_1 v_i^{(1)} & S_1 v_i^{(2)} \end{bmatrix}^{-1} \tag{54}$$

Hence the impedance matrix can is calculated as

$$Z = \begin{bmatrix} -\frac{T_{22}}{T21} & -\frac{1}{T21} \\ \frac{T_{12}T_{21}-T_{11}T_{22}}{T21} & -\frac{T_{11}}{T21} \end{bmatrix} \tag{55}$$

## References


[1] Sergei Tretyakov, *Analytical modeling in applied electromagnetics*, Artech House, 2000.

[2] Xuchen Wang, et. al., *Systematic design of printable metasurfaces: Validation through reverse-offset printed millimeter-wave absorbers*, IEEE Transactions on Antennas and Propagation 66 (3), 1340-1351, 2018.
